# Supplementary material for: Open-Canopy: Towards Very High Resolution Forest Monitoring
Source: arXiv:2407.09392 source file (2024-12-11)
Supplement: Supplementary file 2 [file supmat_change_2.tex]

%auto-ignore
\centering
\begin{tabular}{c@{\,}c@{\,}c@{\,}c@{\,}c@{\,}c}
\begin{subfigure}{.18\textwidth}
  \begin{tikzpicture}
    \node[anchor=south west,inner sep=0] (image) at (0,0) {\includegraphics[width=\textwidth]{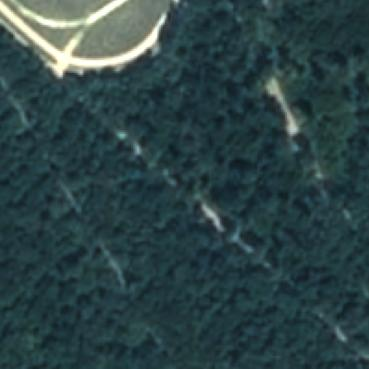}
    };
     \begin{scope}[x={(image.south east)},y={(image.north west)}]
     \node[fill=none, draw=none, text=black] (n1) at (0.145,0.89) {\includegraphics[width={0.1}\textwidth]{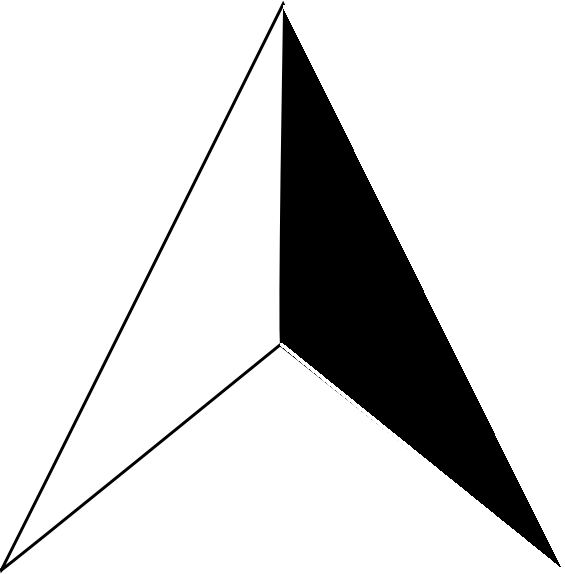}} ;
      \node[fill=none, draw=none, text=black] (n1) at (0.145,0.75) {\contour{white}{\scriptsize N}} ;
      \draw[-, fill=white, text=black, draw=white, ultra thick] (0.07,0.10) -- (0.22,0.10);
      \draw[<->, fill=white, text=black, draw=black,  thick] (0.05,0.10) -- (0.24,0.10);
      \draw[-, draw=black, thick] (0.145,0.10) -- (0.145,0.05);
      \node[fill=none, text=black, draw=none] at (0.145,0.18)  {\tiny  \contour{white}{\bf 50m}};
     \end{scope}
\end{tikzpicture}
\caption{\scriptsize VHR year 2022 }
\label{fig:supmat-change:a}
\end{subfigure}
&
\begin{subfigure}{.18\textwidth}
\includegraphics[width=\textwidth]{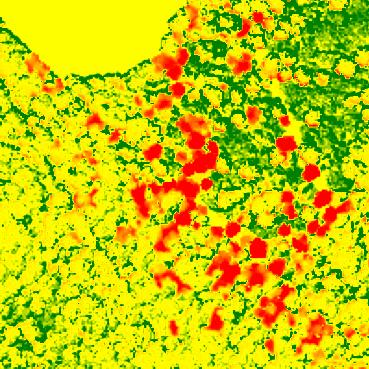}
\caption{\scriptsize  ALS change map }
\label{fig:supmat-change:b}
\end{subfigure}
&
\begin{subfigure}{.18\textwidth}
\includegraphics[width=\textwidth]{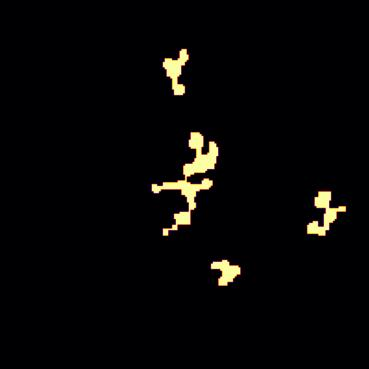}
\caption{\scriptsize ALS change mask }
\label{fig:supmat-change:d}
\end{subfigure}
\\
\begin{subfigure}{.18\textwidth}
\includegraphics[width=\textwidth]{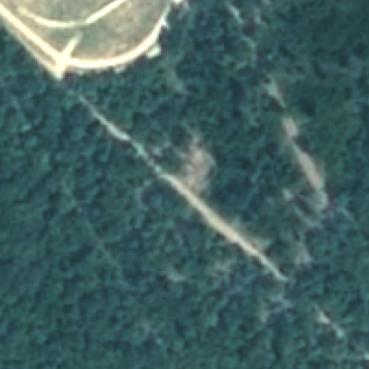}
\caption{\scriptsize VHR year 2023 }
\label{fig:supmat-change:f}
\end{subfigure}
&
\begin{subfigure}{.18\textwidth}
\includegraphics[width=\textwidth]{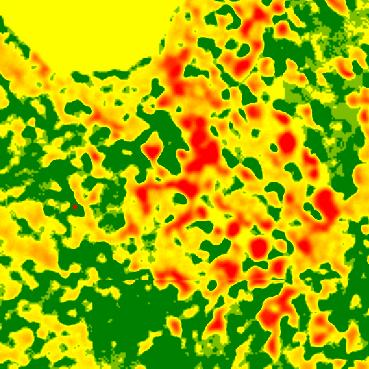}
\caption{\scriptsize {Our change map}  }
\label{fig:supmat-change:g}
\end{subfigure}
&
\begin{subfigure}{.18\textwidth}
\includegraphics[width=\textwidth]{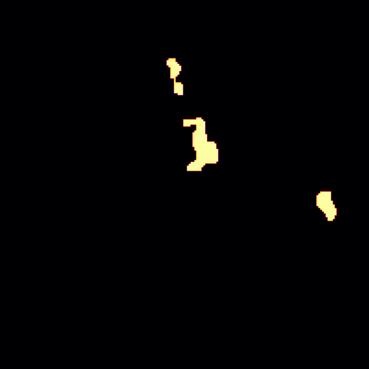}
\caption{\scriptsize Our change mask}
\label{fig:supmat-change:i}
\end{subfigure}
&
\multirow[t]{2}{*}[+0.925cm]{
\hspace{-0.5cm}
\colorbargrowth{3.85cm}
}
\end{tabular}
